# Supplementary material for: Bayesian Active Learning for Sim-to-Real Robotic Perception
Source: arXiv:2109.11547 source file (2022-08-01)
Supplement: Supplementary file 1 [file appendix.tex]

%\section*{APPENDIX}
%Appendixes should appear before the acknowledgment.
